# Supplementary material for: Make Pixels Dance: High-Dynamic Video Generation
Source: arXiv:2311.10982 source file (2023-11-18)
Supplement: Supplementary file 1 [file 6_appendix.tex]

\newpage

pass
